# Supplementary material for: A Maximum Matching Algorithm for Basis Selection in Spectral Learning
Source: arXiv:1706.02857 source file (2017-06-09)
Supplement: Supplementary file 1 [file supplementary.pdf]

# Supplementary Material: A Maximum Matching Algorithm for Basis Selection in Spectral Learning

**Ariadna Quattoni** and **Xavier Carreras** and **Matthias Gallé**
Xerox Research Centre Europe (XRCE)
Meylan, France
{ariadna.quattoni,xavier.carreras,matthias.galle}@xrce.xerox.com

This is supplementary material to the paper by Quattoni et al. [2017].

## A Experimental Validation of the Weak Matching Property

Ideally, we would not have to assume the *matching property* and instead we could provide theoretical guarantees for the maximum gap between the structural and numeric rank of a matrix. Unfortunately, because of the discrete nature of the structural rank, deriving useful bounds for this gap has been shown to be a hard theoretical challenge Hoffman and McCormick [1982]. Thus to provide validation for our assumption we resorted to an empirical evaluation of the gap on a wide range of sequence modeling datasets. For each dataset we do the following:

1. Compute the corresponding Hankel Matrix for a certain moment size $T$.
2. Compute the structural rank and a corresponding max-matching sub-matrix.
3. Compute the numeric rank of the max-matching sub-matrix.

Table 1 shows the results. We observe that for all datasets the percentual gap is small. We thus conclude that, in practice, the weak matching property is a reasonable assumption in real data.

## B Synthetic Experiments for the Fast Augmenting Path Algorithm

A theoretical analysis of the Fast Augmenting Path Algorithm (presented in Section 4 of the main paper) is challenging. While each iteration is never worse than the baseline iteration (the checks can be done in time $\mathcal{O}(|E|)$ assuming a bitset implementation of sets), it may well be that none of the shifted pairs are free, and therefore only add computation without improving the matching.

We therefore compared its execution time empirically on synthetic data. Random sequences were generated with different alphabet size, and different average length (we sampled from a Gaussian distribution with a variance of 0.5). The respective times are plotted in Figure 1 for different alphabet sizes ($|\Sigma|$) and mean lengths ($\mu_{length}$).

The proposed solution is always better, with increased speed-up with increasing mean length (the average speed-up over all plots goes from 1.18 to 2.66), and with a smaller slope. Both implementations are probably sub-optimal and done in `python`. However, we believe these conclusions carry on to more sophisticated implementations, as any improvement will affect both versions (arguably not equally, as the baseline runs the augmenting path procedure more often).

## References

A.J. Hoffman and S. T. McCormick. A fast algorithm that makes matrices optimally sparse. Technical Report 13, Stanford University Systems Optimization Laboratory Report, 1982.

Ariadna Quattoni, Xavier Carreras, and Matthias Gallé. A maximum matching algorithm for basis selection in spectral learning. In *Proceedings of the 20th International Conference on Artificial Intelligence and Statistics (AISTATS)*, volume 54 of *JMLR Proceedings*, 2017.

Table 1: Empirical measure of the gap between structural and numerical rank of Hankel matrices.

| Data Type | Source | $T$ | Hankel Size | S-Rank | N-Rank |
|---|---|---|---|---|---|
| NLP (character level LM) | Penn Treebank | 7 | 1,007,128 | 13,956 | 12,475 |
| NLP (simplified PoS tags) | Penn Treebank | 5 | 52,450 | 313 | 312 |
| NLP (character level LM) | War and Peace | 7 | 1,215,705 | 26,815 | 24,305 |
| NLP (English verbs) | SPiCe | 7 | 52,474 | 3,845 | 3,130 |
| NLP (character level LM) | SPiCe | 7 | 922,539 | 13,823 | 12,363 |
| Biology (protein family PF1385) | SPiCe | 6 | 1,492,673 | 9,179 | 9,117 |
| NLP (spanish simplified POS tags) | SPiCe | 7 | 581,217 | 17,951 | 16,480 |
| Biology (protein family PF00400) | 6 | SPiCe | 1,260,878 | 9,082 | 8,931 |
| NLP (text normalizarion) | SPiCe | 7 | 348,274 | 32,277 | 26,054 |

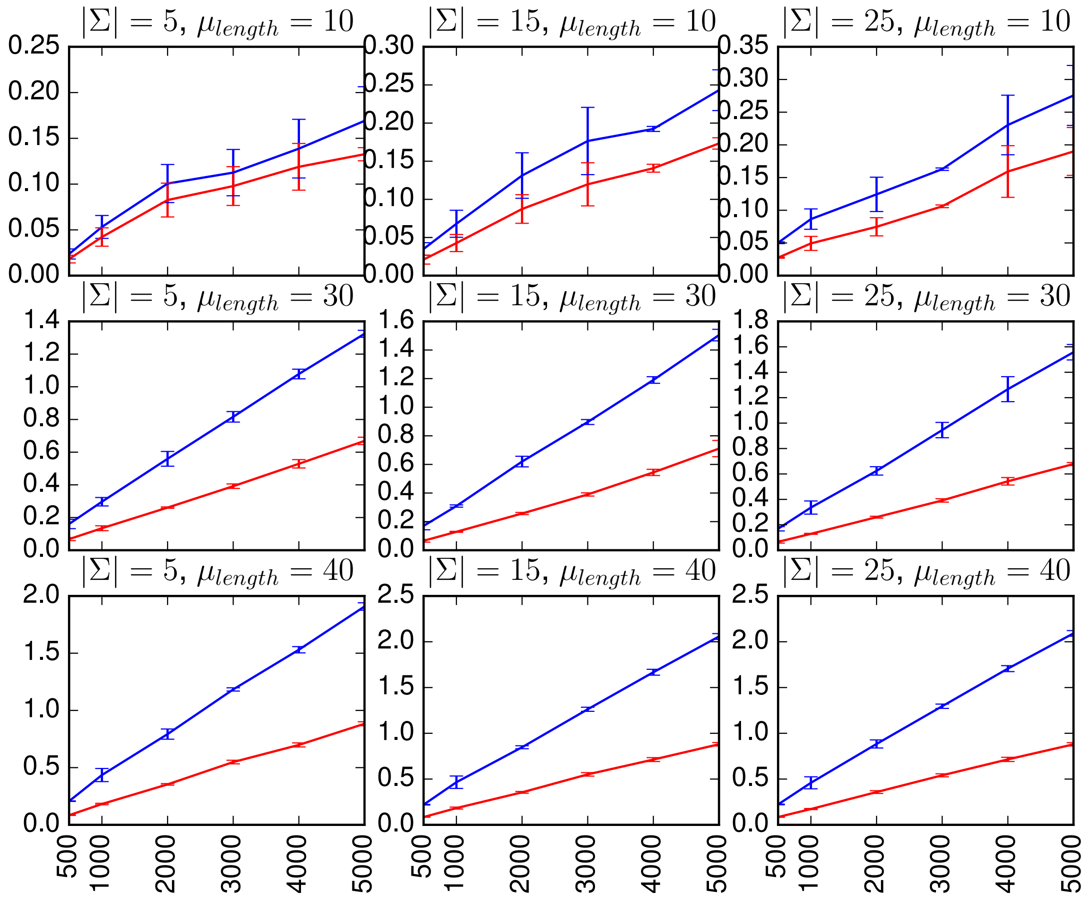


Figure 1: Average and standard deviation (10 iterations) of the time spent for the baseline (in blue) and our proposed solution (in red). $x$-axis is the number of sequences, $y$-axis time in seconds.
